# Supplementary material for: Les Houches 2019: Physics at TeV Colliders: Standard Model Working Group Report
Source: arXiv:2003.01700 source file (2020-03-03)

channel fractions

quark jet

qq2qq  
qq2gg  
qg2qq  
gg2qq  
gg2gg

$|y| < 0.5$

$p_t$

$\sqrt{s}=13$  TeV, CT14nlo, anti- $k_t(0.4)$

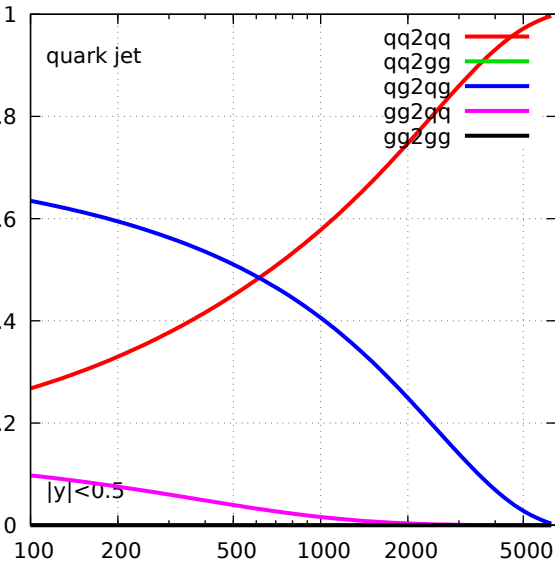

channel fractions

gluon jet

$|y| < 0.5$

qq2qq  
qq2gg  
qg2qq  
gg2qq  
gg2gg

$\sqrt{s}=13$  TeV, CT14nlo, anti- $k_t(0.4)$

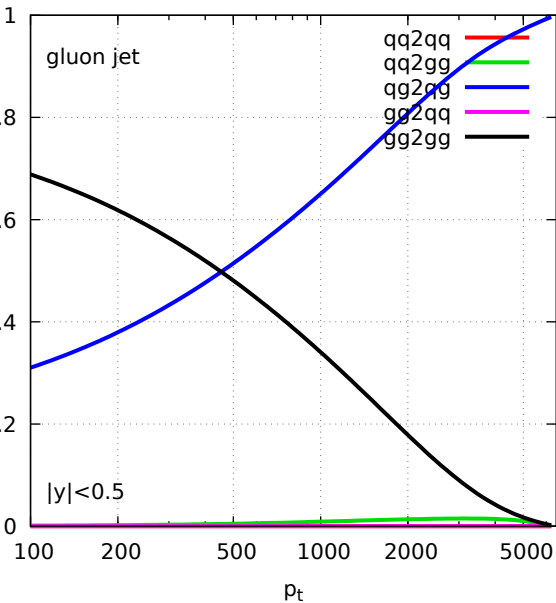

channel fractions

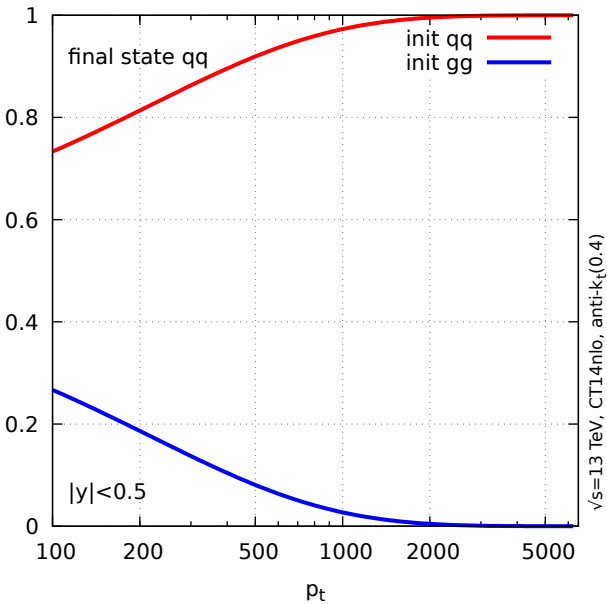

channel fractions

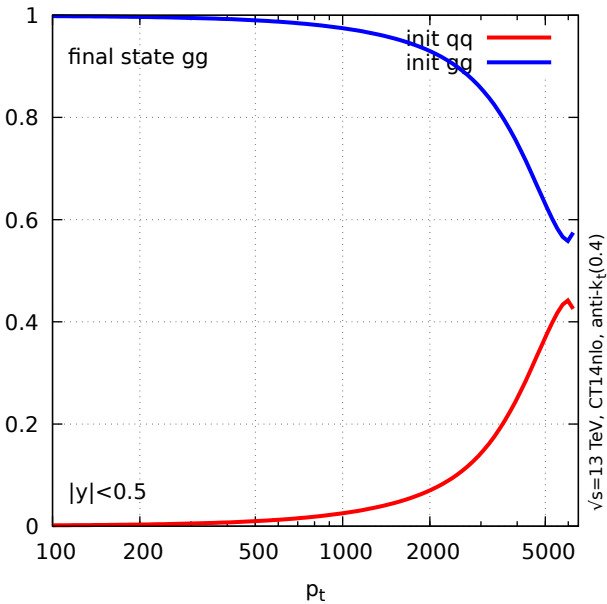

channel fractions

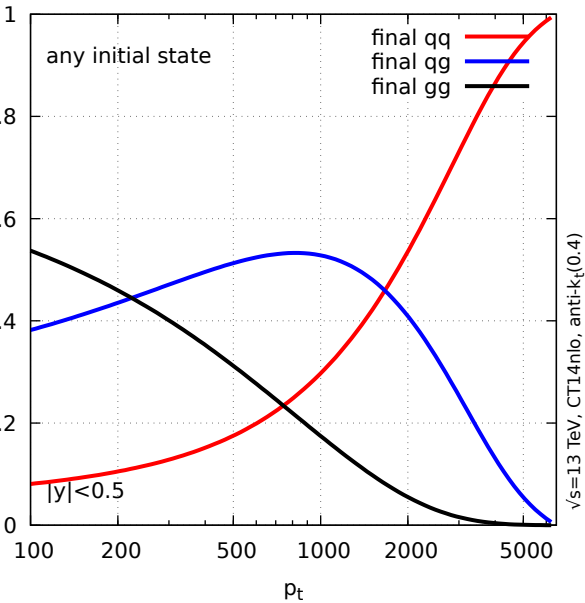

channel fractions

quark jet

qq2qq  
qq2gg  
qg2qq  
gg2qq  
gg2gg

$|y| < 4.5$

$p_t$

$\sqrt{s}=13$  TeV, CT14nlo, anti- $k_t(0.4)$

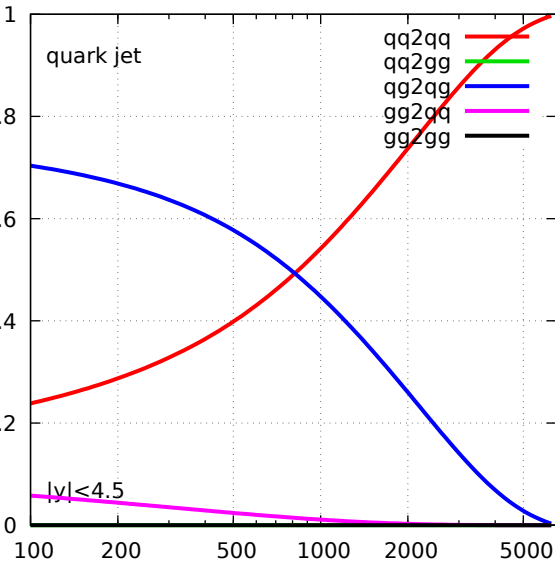

channel fractions

gluon jet

$|y| < 4.5$

qq2qq  
qq2gg  
qg2qq  
gg2qq  
gg2gg

$\sqrt{s}=13$  TeV, CT14nlo, anti- $k_t(0.4)$

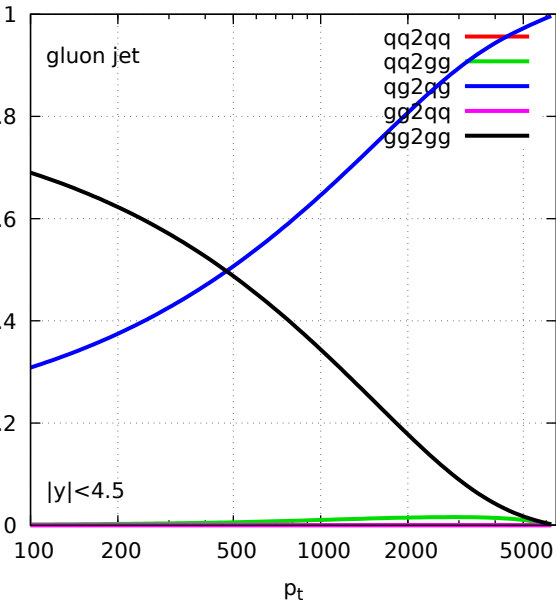

channel fractions

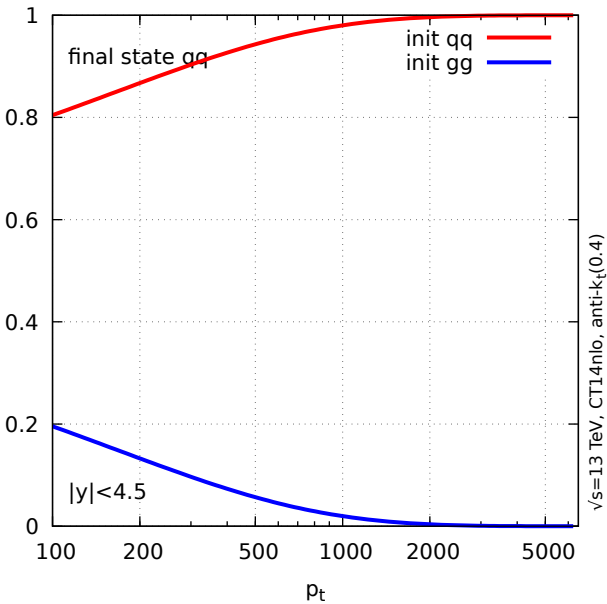



channel fractions

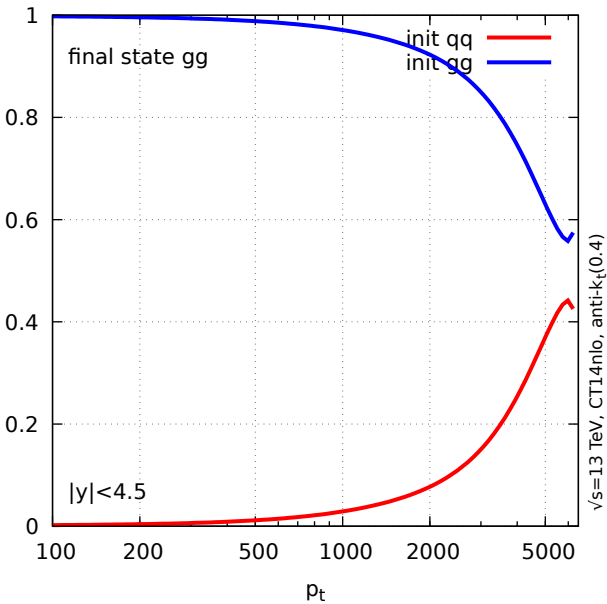

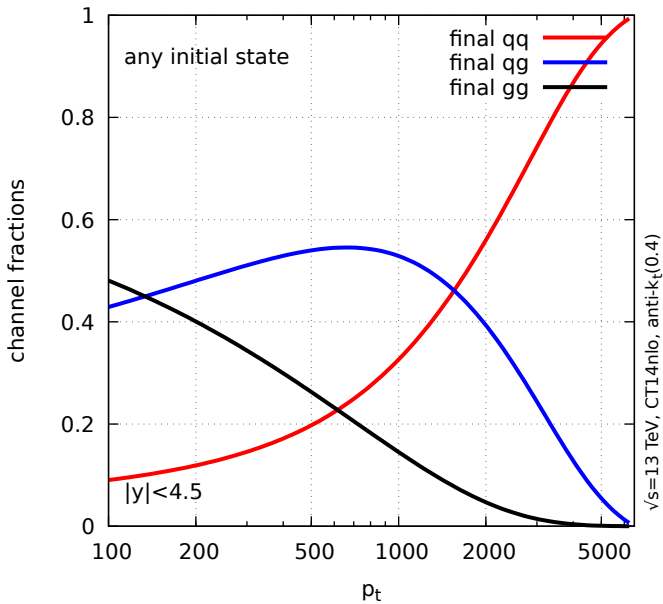

Supplement: Supplementary file 1 [file fractions.pdf]
