# Supplementary material for: Les Houches 2019: Physics at TeV Colliders: Standard Model Working Group Report
Source: arXiv:2003.01700 source file (2020-03-03)

PDF uncertainty  $v$  (ideal) tagging purity

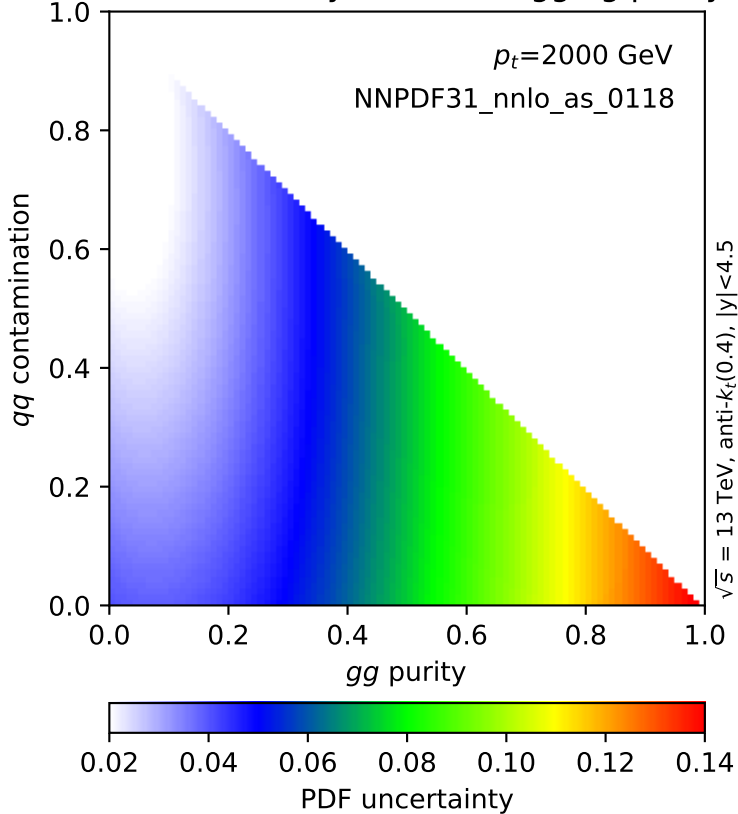

# PDF uncertainty v (ideal) tagging purity

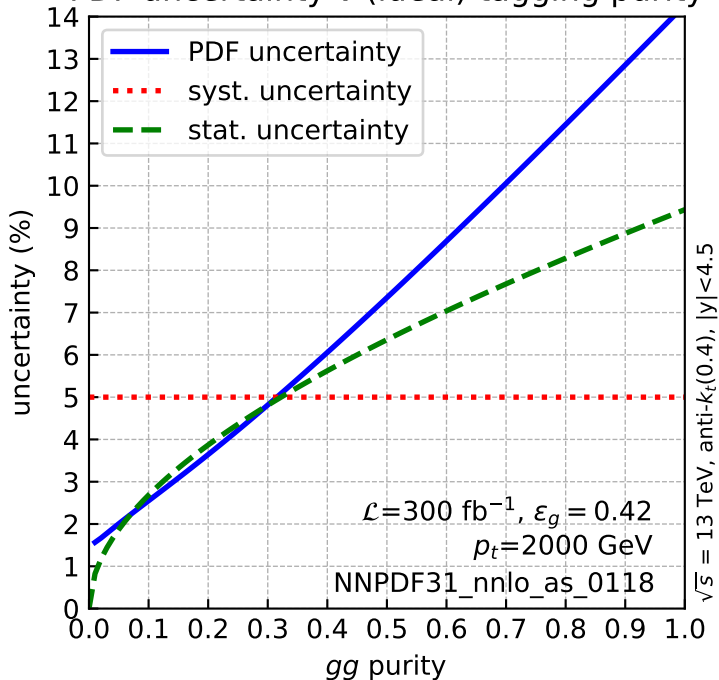

# quark mistag rate

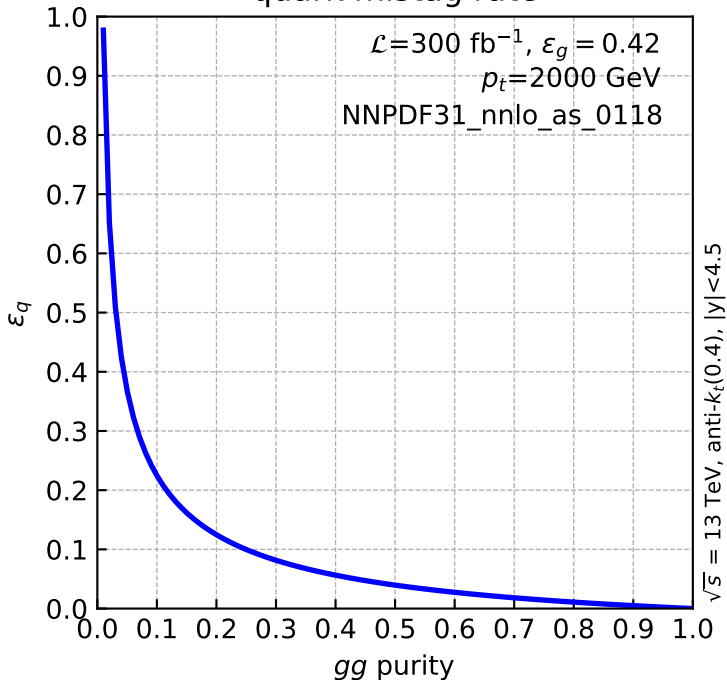

# ROC curves for a few selected taggers

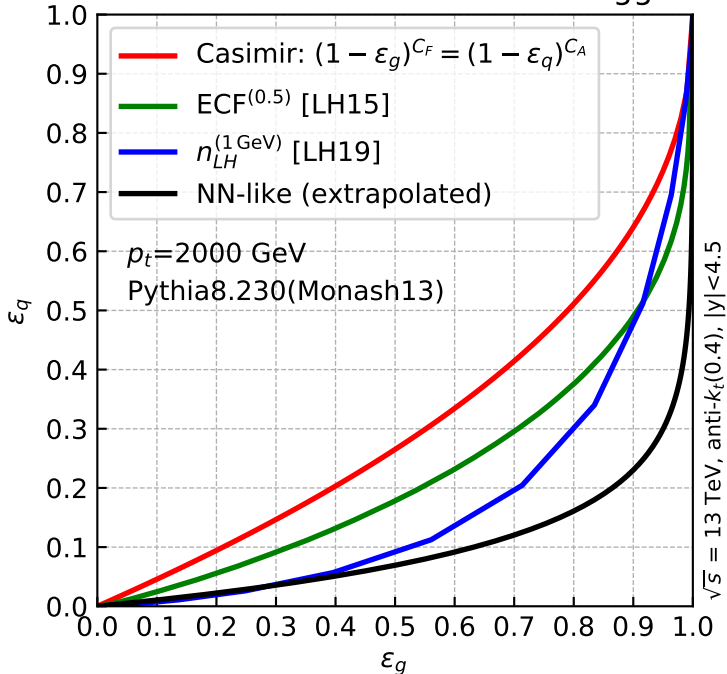

# Uncertainties for a few selected taggers

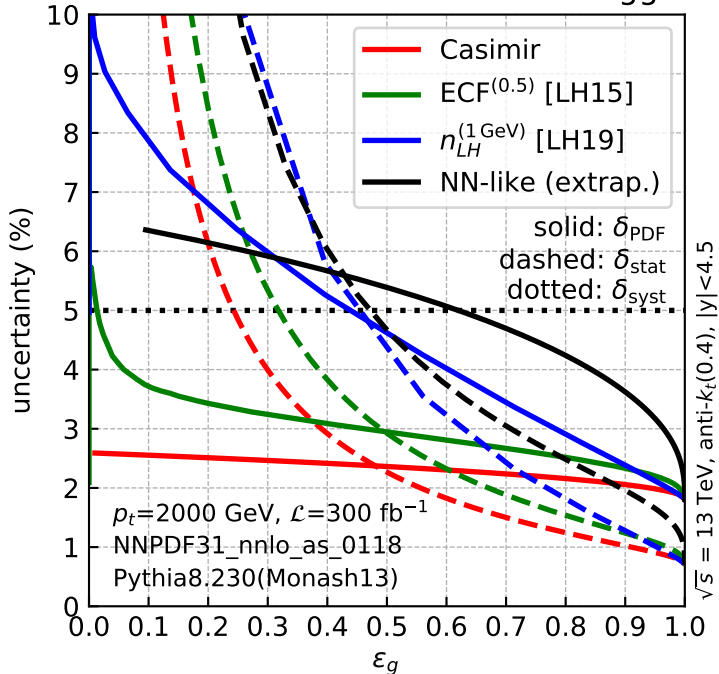

Supplement: Supplementary file 2 [file performance-plots.pdf]
